# Supplementary material for: Graph Balancing with Orientation Costs
Source: arXiv:2106.05939 source file (2021-06-10)
Supplement: Supplementary file 1 [file AdditionalIntegralityGaps.tex]

We show an integrality gap (to LP3 or the more strong relaxation) that shows that to GB with light hyper edges, any rounding algorithm that is a $c$-approximation to the costs where $c<2$, has to be at least 1.75 approximation to the makespan.
{\color{red}This is not accurate and not interesting. It shows that if you want to get below 2 in costs then have to be at least $1.75-\epsilon$ in the makespan. But there is an integrality gap of 1.75 so not interesting. The integrality gap of 1.75 is similar to this one. just need two copies of the path and connect the $u$ vertices with each other in a light edge weight with weight $0.5$. Maybe it is interesting? because the 1.75 gap to \sGB is not valid to \LPstong with Set constraints of size 2.}
\begin{figure}[H]
	\includegraphics[width=\linewidth]{Integrality Gap3.jpeg}
	\caption{Integrality Gap3}
\end{figure}
